# Supplementary material for: Geometric Probing for Algorithm Selection in Continuous Black-Box Optimization
Source: arXiv:2604.09095 source file (2026-10-07)
Supplement: Supplementary file 1 [file appendix.tex]

\documentclass[lettersize,journal]{IEEEtran}

% ---------- Packages ----------
\usepackage{amsmath,amssymb,amsfonts}
\usepackage{graphicx}
\usepackage{booktabs}
\usepackage{multirow}
\usepackage{array}
\usepackage{xcolor}
\usepackage{url}
\usepackage{hyperref}
\usepackage{rotating}

% If you use subfigures:
% \usepackage{subcaption}

% If you use algorithms:
% \usepackage{algorithm}
% \usepackage{algorithmic}

% ---------- Supplementary numbering ----------
\renewcommand{\thesection}{S\Roman{section}}
\renewcommand{\thesubsection}{S\Roman{section}.\Alph{subsection}}
\renewcommand{\thefigure}{S\arabic{figure}}
\renewcommand{\thetable}{S\arabic{table}}
\renewcommand{\theequation}{S\arabic{equation}}

% If using algorithms:
% \renewcommand{\thealgorithm}{S\arabic{algorithm}}

% ---------- Metadata ----------
\title{Supplementary Material}

% \author{Anonymous Author(s)}

\begin{document}

\maketitle

\input{sections/appendix}

% Original Appendix C here.

\end{document}
