# Supplementary material for: Geometric Probing for Algorithm Selection in Continuous Black-Box Optimization
Source: arXiv:2604.09095 source file (2026-10-07)
Supplement: Supplementary file 2 [file appendix_legacy.tex]

\appendix
% \section{Supplementary Materials}

\subsection{Geometric probing}

\begin{figure*}[t]
    \centering
    % \includegraphics[width=0.98\linewidth]{img/GECCO2026/plots_over_problems.pdf}
    \includegraphics[width=0.98\linewidth]{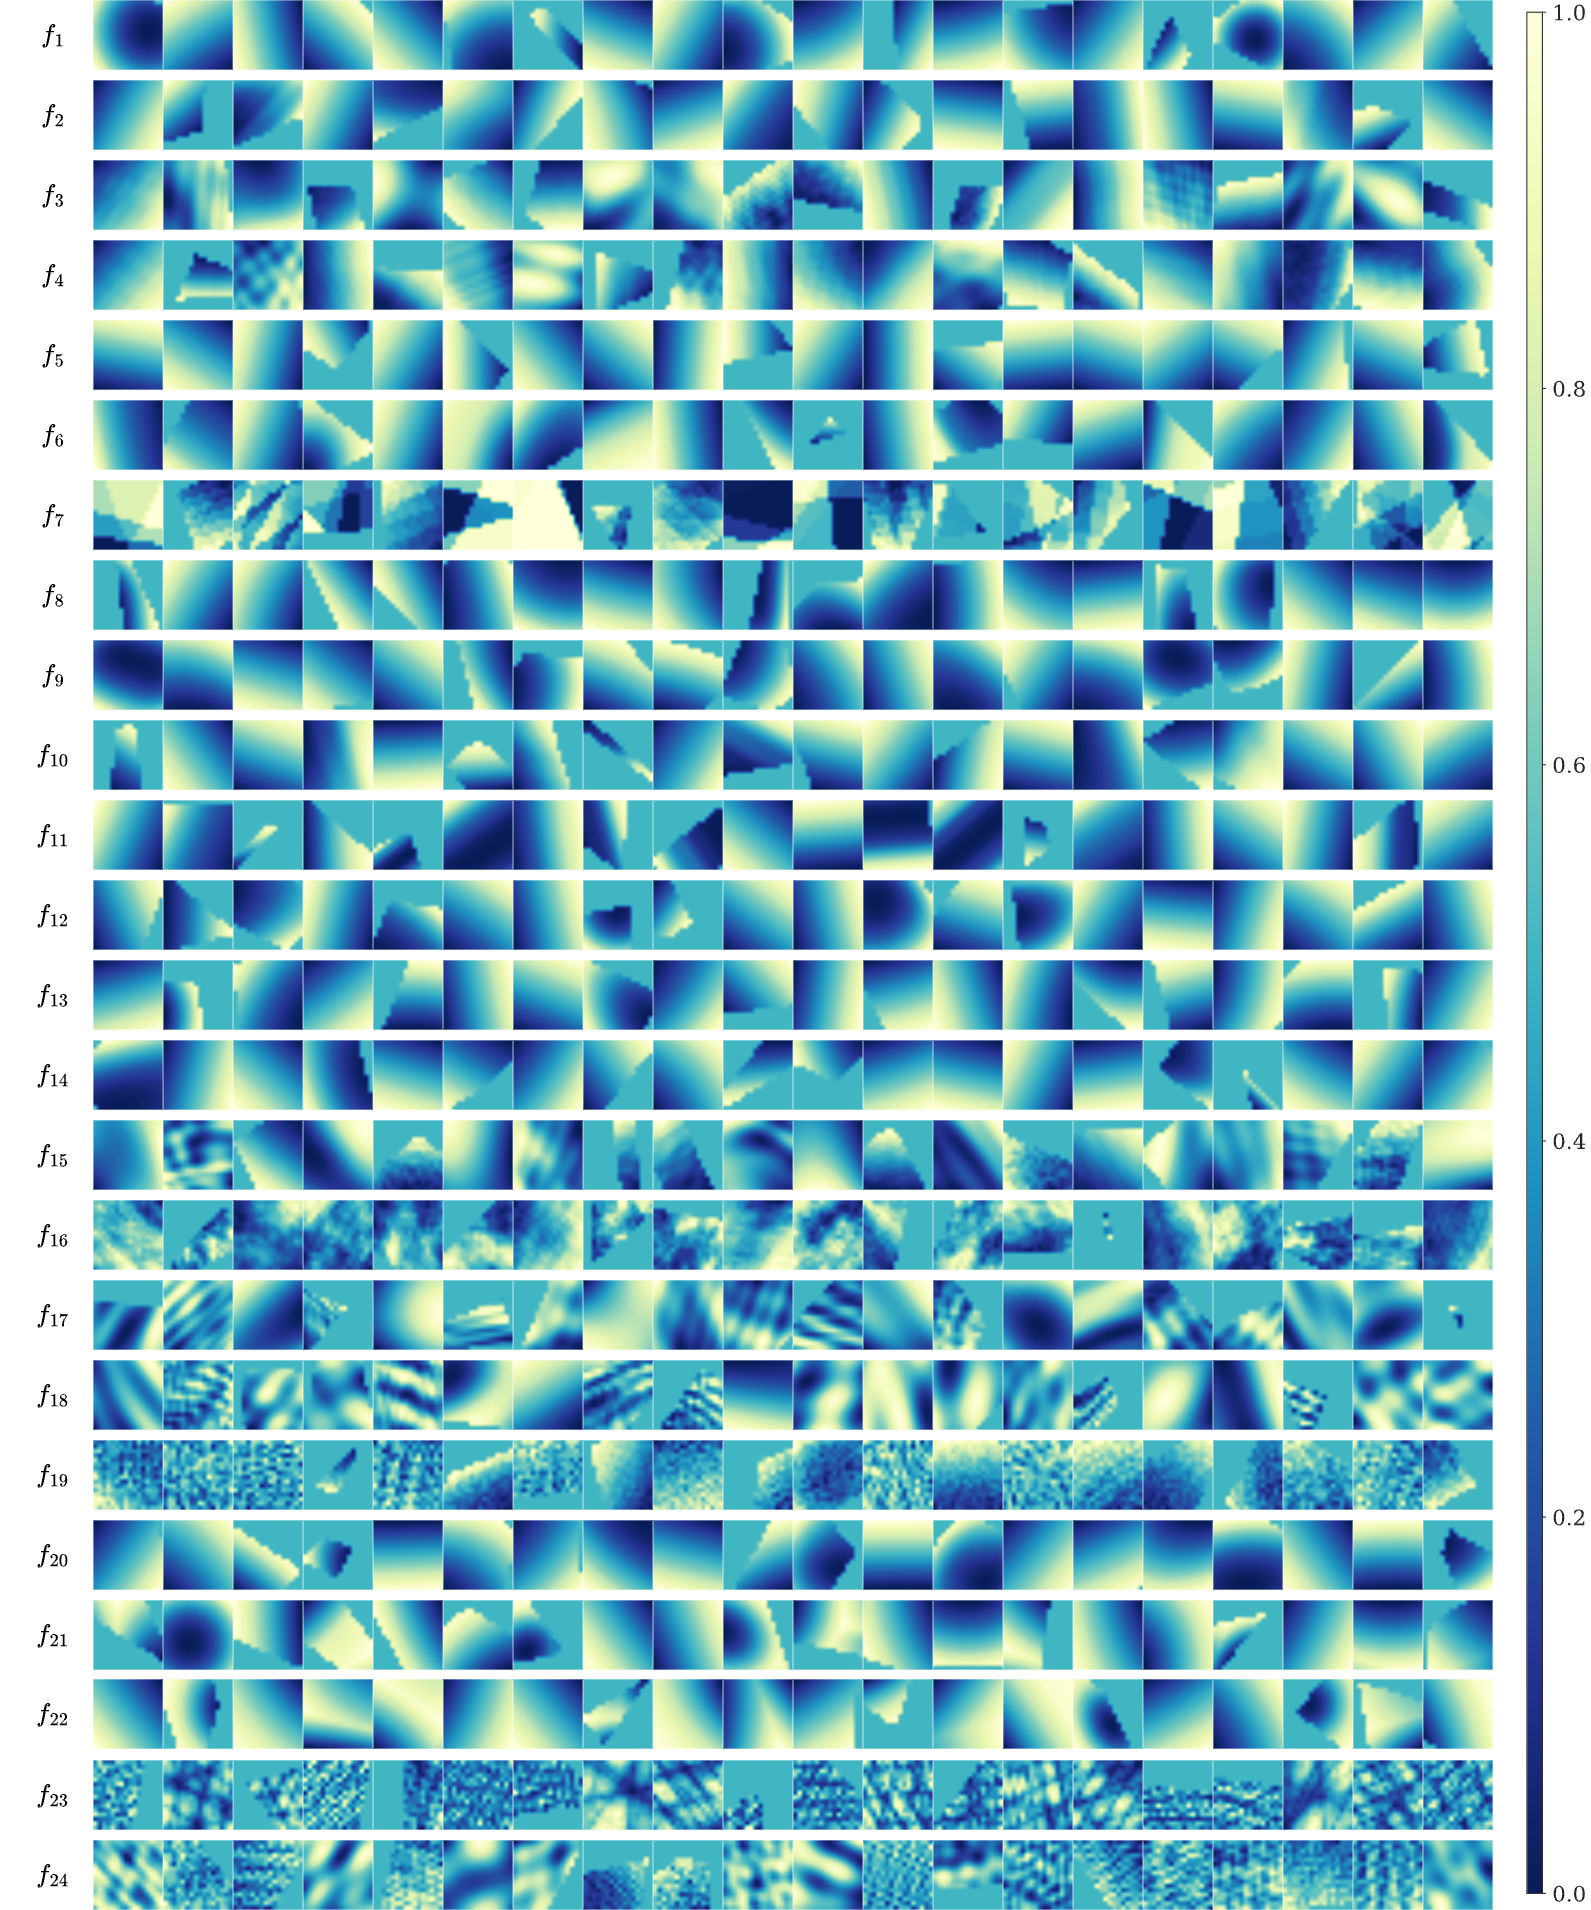}
    \caption{Twenty sampled, normalized slices (value channel) of resolution $8\times 8$ for each of the 24 BBOB functions, under dimension \(d =10\).}
    \label{fig:plots_over_problems}
\end{figure*}

\subsubsection{Qualitative examples across problems}
Figure~\ref{fig:plots_over_problems} shows representative normalized value maps across the 24 BBOB functions. 
The examples illustrate that coarse \(8\times8\) slices can retain visibly different local geometric patterns across function families, including smooth trends, oscillatory structure, boundary truncation, and multimodal variation. 
% Only the value channel is shown here; the corresponding validity-mask mechanism is illustrated in Figure~\ref{fig:plot_mask_demo}.

\begin{table}
    \centering
    \caption{Average wall-clock time (s) to generate the input for a set of 128 slices across resolutions and dimensions (number of function evaluations per slice in parentheses).}
    \label{tab:probing_cost}
    \begin{tabular}{c|cccc}
    \toprule
    \textbf{Resolution (\#evaluations)} & \multicolumn{4}{c}{\textbf{Dimension}} \\
    \cmidrule{2-5}
     & 2 & 3 & 5 & 10 \\
    \midrule
    $8\times8\ (8.1k)$     & 0.067 & 0.068 & 0.063 & 0.066 \\
    $16\times16\ (32.8k)$  & 0.178 & 0.261 & 0.200 & 0.180 \\
    $32\times32\ (131.1k)$ & 0.550 & 0.589 & 0.578 & 0.613 \\
    $64\times64\ (524.3k)$ & 2.111 & 2.213 & 2.195 & 2.346 \\
    \bottomrule
    \end{tabular}
\end{table}

\subsubsection{Probing cost}
Table~\ref{tab:probing_cost} reports the average wall-clock time required to construct 
\(\{(X_i,M_i,\ell_i,\Delta_i,q_i)\}_{i=1}^{128}\) for different slice resolutions and dimensions. 
In this synthetic BBOB setting, input generation remains below one second up to resolution \(32\times32\), and rises to approximately \(2.1\)--\(2.3\) seconds at \(64\times64\). 
The variation across dimensions is small relative to the variation across resolutions, indicating that the measured cost is driven mainly by the number of within-slice evaluations. 
These timings, however, should not be interpreted as deployment costs for expensive black-box objectives, as they only measure overhead on cheap, synthetic benchmark functions.

\subsection{Instantiated architecture}
\label{app:architecture}

The architecture follows the encoder--aggregator--selector decomposition in the main text. 
Here we specify the omitted widths and layer types.

The shared per-slice visual encoder uses three convolutional blocks with channel widths
\[
1 \rightarrow 32 \rightarrow 64 \rightarrow 128 .
\]
Each block contains two \(3\times3\) convolutions with padding \(1\), each followed by ReLU. 
After the first two blocks, both the feature map and the validity mask are downsampled by \(2\times2\) max-pooling with stride \(2\). 
The final spatial feature map is reduced to a slice embedding by masked spatial attention using a learned \(1\times1\) scoring convolution. 
Thus, the visual slice embedding dimension is \(C_X=128\).

The log-transformed slice-side statistics \((\ell_i,\Delta_i,q_i)\) are embedded by a linear map 
\[
\mathbb{R}^3 \rightarrow \mathbb{R}^{16},
\]
so \(C_\xi=16\). 
After concatenation with the visual slice embedding, slice representations are aggregated across the \(k\) sampled slices by attention pooling with a shared linear scorer.

The ambient dimension is encoded by a linear map 
\[
\mathbb{R} \rightarrow \mathbb{R}^{4}
\]
applied to \(\log d\), so \(C_d=4\). 
The final instance representation therefore has dimension
\[
C_X + C_\xi + C_d = 128 + 16 + 4 = 148 .
\]

After dropout with rate \(0.2\), this representation is passed to a prediction head implemented as a three-layer MLP with widths
\[
148 \rightarrow 256 \rightarrow 128 \rightarrow |\mathcal A|,
\]
with ReLU activations between hidden layers.

\subsection{Supplementary results}\label{app:analysis_supplements}

\begin{figure*}[t]
    \centering
    \includegraphics[width=\linewidth]{img/IEEETEC2026_GeoPAS/supplementary_random.pdf}
    \caption{Supplementary analyses under the Random protocol. 
    The panels report selection-score sensitivity, selection-frequency behavior, probing-budget robustness, and realized \(\mathrm{relERT}\)/survival-curve behavior. 
    Random closely follows the LIO pattern, supporting its interpretation as a leakage-safe within-suite sanity check rather than a qualitatively separate transfer setting.}
    \label{fig:supplementary-random}
\end{figure*}

\subsubsection{Results under Random}
\label{app:random-results}

Figure~\ref{fig:supplementary-random} collects the supplementary Random-protocol analyses corresponding to the main-text LIO/LPO results. 
The selection-score grid shows the same adaptivity--robustness trade-off observed under LIO: learned-dominant settings improve typical rankings, while shrinkage is needed to stabilize mean behavior. 
The budget analysis likewise follows the within-suite pattern, with additional views generally improving median and upper-tail performance until saturation. 
The distributional and selection-frequency plots also mirror LIO, with GeoPAS shifting mass toward lower \(\mathrm{relERT}\) and without introducing the LPO-specific extreme-tail behavior. 
These results justify keeping Random in the appendix for completeness while using LIO and LPO as the main contrast between within-suite behavior and problem-family transfer.

% \begin{sidewaystable*}[p]
\begin{table*}
\centering
\caption{Supplementary diagnostic results under LIO for GeoPAS under the main configuration, the learned-only selection score \(\alpha=0\), the prior-heavy configuration \((\gamma,\alpha)=(0.8,0.8)\), and the no-dimension-conditioning setting.}
\label{tab:supplementary-diagnostics_lio}
\resizebox{\linewidth}{!}{%
\begin{tabular}{cc|cccc|cccc|cccc}
\toprule
\textbf{F. group} & \textbf{D} & \multicolumn{12}{c|}{\textbf{LIO}} \\
\cmidrule{3-14}
& & \multicolumn{4}{c|}{\textbf{Mean}} & \multicolumn{4}{c|}{\textbf{Median}} & \multicolumn{4}{c|}{\textbf{P90}}   \\
\cmidrule{3-6}\cmidrule{7-10}\cmidrule{11-14}
& & GeoPAS & $\alpha=0$ & $\gamma=.8,\alpha=.8$ & no-$\psi_d$ & GeoPAS & $\alpha=0$ & $\gamma=.8,\alpha=.8$ & no-$\psi_d$ & GeoPAS & $\alpha=0$ & $\gamma=.8,\alpha=.8$ & no-$\psi_d$ \\
\midrule
\multirow{5}{*}{f1-f5} & 2 & 2.28 & 2.35 & 2.25 & 2.59 & 1.95 & 1.00 & 1.95 & 1.95 & 4.10 & 3.20 & 4.10 & 4.10 \\
 & 3 & 14.39 & 54.89 & 60.96 & 142.65 & 2.64 & 1.13 & 2.64 & 2.64 & 13.68 & 12.26 & 13.68 & 72.09 \\
 & 5 & 11.77 & 20.62 & 11.99 & 12.45 & 1.64 & 1.06 & 1.64 & 1.64 & 51.82 & 3.79 & 51.82 & 53.15 \\
 & 10 & 3.26 & 198.31 & 3.00 & 737.28 & 2.94 & 1.16 & 2.94 & 2.94 & 6.17 & 7.24 & 5.20 & 7.24 \\
\cmidrule{2-14}
 & all & 7.93 & 69.04 & 19.55 & 223.74 & 2.03 & 1.05 & 2.39 & 2.23 & 11.55 & 7.14 & 11.76 & 13.68 \\
\midrule
\multirow{5}{*}{f6-f9} & 2 & 1.26 & 1.75 & 1.20 & 1.23 & 1.08 & 1.31 & 1.08 & 1.11 & 1.60 & 1.88 & 1.60 & 1.60 \\
 & 3 & 1.07 & 3.54 & 1.05 & 1.10 & 1.06 & 1.04 & 1.05 & 1.05 & 1.07 & 1.46 & 1.07 & 1.07 \\
 & 5 & 1.33 & 1.20 & 1.42 & 1.30 & 1.27 & 1.06 & 1.27 & 1.27 & 1.55 & 1.68 & 2.04 & 1.79 \\
 & 10 & 1.36 & 1.30 & 1.58 & 1.30 & 1.20 & 1.19 & 1.38 & 1.20 & 1.72 & 1.96 & 2.57 & 1.61 \\
\cmidrule{2-14}
 & all & 1.26 & 1.95 & 1.32 & 1.23 & 1.07 & 1.09 & 1.09 & 1.07 & 1.60 & 1.76 & 1.72 & 1.61 \\
\midrule
\multirow{5}{*}{f10-f14} & 2 & 1.00 & 1.02 & 1.01 & 1.03 & 1.00 & 1.00 & 1.00 & 1.00 & 1.00 & 1.00 & 1.00 & 1.00 \\
 & 3 & 1.03 & 98.85 & 1.05 & 1.12 & 1.00 & 1.00 & 1.00 & 1.00 & 1.01 & 1.01 & 1.01 & 1.01 \\
 & 5 & 1.33 & 196.76 & 1.75 & 1.15 & 1.01 & 1.01 & 1.03 & 1.00 & 2.07 & 1.17 & 3.50 & 1.32 \\
 & 10 & 1.49 & 196.84 & 1.77 & 1.24 & 1.09 & 1.01 & 1.10 & 1.00 & 2.80 & 1.36 & 3.83 & 1.50 \\
\cmidrule{2-14}
 & all & 1.21 & 123.37 & 1.40 & 1.14 & 1.00 & 1.00 & 1.00 & 1.00 & 1.37 & 1.27 & 2.69 & 1.13 \\
\midrule
\multirow{5}{*}{f15-f19} & 2 & 1.90 & 100.39 & 1.95 & 2.01 & 1.73 & 1.00 & 1.73 & 1.73 & 3.26 & 1.96 & 3.26 & 3.26 \\
 & 3 & 2.84 & 931.60 & 2.83 & 3.11 & 2.13 & 1.11 & 2.61 & 2.20 & 3.85 & 3.85 & 3.58 & 5.23 \\
 & 5 & 4.34 & 1029.88 & 4.44 & 3.97 & 2.23 & 1.05 & 2.23 & 2.23 & 14.86 & 6.74 & 14.86 & 14.86 \\
 & 10 & 2.31 & 637.26 & 2.18 & 246.95 & 1.00 & 1.00 & 1.00 & 1.00 & 5.57 & 1.93 & 5.57 & 5.57 \\
\cmidrule{2-14}
 & all & 2.85 & 674.78 & 2.85 & 64.01 & 1.99 & 1.00 & 2.03 & 1.99 & 5.00 & 3.67 & 5.57 & 5.57 \\
\midrule
\multirow{5}{*}{f20-f24} & 2 & 2.44 & 1.32 & 6.20 & 3.06 & 1.54 & 1.00 & 1.61 & 1.61 & 3.69 & 1.51 & 12.05 & 7.04 \\
 & 3 & 3.14 & 1.38 & 8.11 & 20.83 & 1.67 & 1.01 & 1.67 & 1.67 & 4.22 & 1.76 & 6.23 & 14.33 \\
 & 5 & 1.17 & 1.04 & 1.19 & 1126.46 & 1.00 & 1.00 & 1.00 & 1.00 & 1.77 & 1.08 & 1.77 & 1.77 \\
 & 10 & 1.55 & 50.07 & 1.59 & 197.24 & 1.00 & 1.00 & 1.00 & 1.00 & 2.19 & 1.32 & 2.19 & 2.19 \\
\cmidrule{2-14}
 & all & 2.07 & 13.45 & 4.27 & 336.90 & 1.01 & 1.00 & 1.48 & 1.46 & 2.60 & 1.42 & 6.23 & 3.28 \\
\midrule
\multirow{5}{*}{all} & 2 & 1.80 & 22.18 & 2.58 & 2.01 & 1.46 & 1.00 & 1.52 & 1.46 & 2.92 & 1.95 & 3.26 & 3.26 \\
 & 3 & 4.64 & 226.99 & 15.38 & 35.12 & 1.07 & 1.00 & 1.61 & 1.44 & 5.06 & 2.93 & 5.06 & 5.06 \\
 & 5 & 4.10 & 260.26 & 4.27 & 238.56 & 1.09 & 1.01 & 1.23 & 1.05 & 3.88 & 3.10 & 5.12 & 4.45 \\
 & 10 & 2.02 & 225.73 & 2.04 & 246.61 & 1.16 & 1.00 & 1.32 & 1.05 & 4.06 & 2.42 & 4.19 & 4.45 \\
\cmidrule{2-14}
 & all & 3.14 & 183.79 & 6.07 & 130.58 & 1.19 & 1.00 & 1.40 & 1.17 & 3.96 & 2.64 & 4.10 & 4.10 \\
\bottomrule
\end{tabular}%

}

% \vspace{0.3em}
% \GCColorbar
% \vspace{0.5em}

\end{table*}
% \end{sidewaystable*}


\begin{table*}
\centering
\caption{Supplementary diagnostic results under LPO for GeoPAS under the main configuration, the learned-only selection score \(\alpha=0\), the prior-heavy configuration \((\gamma,\alpha)=(0.8,0.8)\), and the no-dimension-conditioning setting.}
\label{tab:supplementary-diagnostics_lpo}
\resizebox{\linewidth}{!}{%
\begin{tabular}{cc|cccc|cccc|cccc}
\toprule
\textbf{F. group} & \textbf{D}  & \multicolumn{12}{c}{\textbf{LPO}}\\
\cmidrule{3-14}
&    & \multicolumn{4}{c|}{\textbf{Mean}} & \multicolumn{4}{c|}{\textbf{Median}} & \multicolumn{4}{c}{\textbf{P90}}\\
\cmidrule{3-6}\cmidrule{7-10}\cmidrule{11-14}
& & GeoPAS & $\alpha=0$ & $\gamma=.8,\alpha=.8$ & no-$\psi_d$ & GeoPAS & $\alpha=0$ & $\gamma=.8,\alpha=.8$ & no-$\psi_d$ & GeoPAS & $\alpha=0$ & $\gamma=.8,\alpha=.8$ & no-$\psi_d$\\
\midrule
\multirow{5}{*}{f1-f5} & 2 & 2.39 & 3.53 & 2.45 & 2.70 & 1.95 & 1.95 & 1.95 & 1.95 & 4.10 & 4.25 & 4.10 & 4.10\\
 & 3 & 343.87 & 4137.15 & 346.21 & 336.73 & 2.64 & 2.64 & 2.64 & 2.64 & 1765.87 & 13407.35 & 1765.87 & 1765.87\\
 & 5 & 19.86 & 1494.66 & 12.09 & 12.34 & 1.82 & 3.22 & 1.82 & 2.00 & 51.82 & 633.14 & 51.82 & 51.82\\
 & 10 & 52.49 & 2596.49 & 3.54 & 492.95 & 2.94 & 4.01 & 2.94 & 2.94 & 7.24 & 1230.70 & 7.24 & 7.24\\
\cmidrule{2-14}
 & all & 104.65 & 2057.95 & 91.07 & 211.18 & 2.64 & 2.74 & 2.64 & 2.62 & 28.96 & 124.72 & 14.31 & 25.76\\
\midrule
\multirow{5}{*}{f6-f9} & 2 & 3.95 & 375.36 & 1.74 & 6.65 & 1.08 & 1.44 & 1.13 & 1.16 & 2.14 & 38.30 & 4.13 & 3.55\\
 & 3 & 674.98 & 1609.17 & 1.57 & 1591.65 & 1.06 & 1.18 & 1.06 & 1.06 & 4.76 & 103.73 & 3.33 & 3.92\\
 & 5 & 2142.51 & 2632.34 & 2.81 & 3792.71 & 1.37 & 1.17 & 1.46 & 1.37 & 12235.31 & 12232.66 & 9.68 & 24460.72\\
 & 10 & 735.43 & 1348.85 & 1.90 & 1713.71 & 1.30 & 1.21 & 1.50 & 1.20 & 3.22 & 1242.55 & 4.07 & 4.35\\
\cmidrule{2-14}
 & all & 889.22 & 1491.43 & 2.01 & 1776.18 & 1.09 & 1.23 & 1.19 & 1.11 & 5.94 & 49.11 & 4.07 & 33.17\\
\midrule
\multirow{5}{*}{f10-f14} & 2 & 1.98 & 54.67 & 2.04 & 2.08 & 1.00 & 1.00 & 1.00 & 1.00 & 3.32 & 2.86 & 4.44 & 4.46\\
 & 3 & 1.69 & 100.01 & 2.69 & 2.14 & 1.00 & 1.00 & 1.78 & 1.01 & 4.84 & 3.07 & 5.82 & 4.84\\
 & 5 & 2.24 & 589.49 & 3.84 & 2.32 & 1.03 & 1.05 & 4.07 & 1.29 & 5.49 & 4.17 & 7.50 & 5.49\\
 & 10 & 51.40 & 3083.57 & 2.75 & 2.10 & 1.50 & 1.24 & 1.79 & 1.13 & 4.97 & 12232.25 & 4.97 & 4.81\\
\cmidrule{2-14}
 & all & 14.33 & 956.94 & 2.83 & 2.16 & 1.01 & 1.01 & 1.37 & 1.03 & 4.88 & 4.01 & 5.49 & 4.85\\
\midrule
\multirow{5}{*}{f15-f19} & 2 & 22.45 & 4283.06 & 21.86 & 112.97 & 2.75 & 4.89 & 2.35 & 2.07 & 86.02 & 24541.29 & 84.64 & 81.45\\
 & 3 & 5.04 & 14778.51 & 3.89 & 101.98 & 3.44 & 12.21 & 3.43 & 2.61 & 11.36 & 36690.30 & 6.35 & 9.38\\
 & 5 & 103.14 & 8076.31 & 4.91 & 249.44 & 2.33 & 5.20 & 2.23 & 2.28 & 14.86 & 36690.30 & 14.86 & 13.77\\
 & 10 & 148.81 & 7339.63 & 2.16 & 2692.87 & 1.00 & 1.51 & 1.00 & 1.00 & 4.07 & 36690.30 & 5.57 & 18.70\\
\cmidrule{2-14}
 & all & 69.86 & 8619.38 & 8.20 & 789.32 & 2.17 & 3.73 & 2.13 & 2.10 & 13.85 & 36690.30 & 14.79 & 12.83\\
\midrule
\multirow{5}{*}{f20-f24} & 2 & 4.96 & 1568.87 & 12.03 & 23.88 & 1.97 & 2.45 & 7.04 & 5.59 & 12.05 & 9.88 & 12.05 & 126.43\\
 & 3 & 33.95 & 1149.70 & 47.32 & 31.29 & 1.68 & 3.58 & 1.68 & 1.68 & 191.82 & 95.23 & 249.05 & 197.54\\
 & 5 & 197.05 & 4697.55 & 2.39 & 2888.43 & 1.00 & 1.03 & 1.00 & 1.00 & 3.45 & 24460.96 & 3.45 & 12234.05\\
 & 10 & 4.17 & 7437.03 & 18.49 & 788.21 & 1.00 & 1.00 & 1.48 & 1.16 & 2.94 & 36690.30 & 106.07 & 3.69\\
\cmidrule{2-14}
 & all & 60.03 & 3713.29 & 20.06 & 932.95 & 1.54 & 1.76 & 1.65 & 1.65 & 8.71 & 24462.28 & 77.36 & 73.36\\
\midrule
\multirow{5}{*}{all} & 2 & 7.28 & 1293.84 & 8.29 & 30.62 & 1.64 & 1.74 & 1.80 & 1.82 & 8.79 & 48.83 & 10.43 & 9.82\\
 & 3 & 192.61 & 4469.31 & 83.61 & 363.64 & 1.76 & 2.13 & 1.89 & 1.95 & 11.36 & 25048.82 & 12.20 & 8.24\\
 & 5 & 424.23 & 3534.14 & 5.31 & 1288.89 & 1.32 & 1.64 & 1.68 & 1.60 & 13.13 & 24477.48 & 12.98 & 26.17\\
 & 10 & 176.08 & 4486.63 & 5.93 & 1113.98 & 1.49 & 1.51 & 1.61 & 1.44 & 4.89 & 36690.30 & 5.57 & 5.75\\
\cmidrule{2-14}
 & all & 200.05 & 3445.98 & 25.78 & 699.28 & 1.58 & 1.73 & 1.76 & 1.64 & 7.84 & 24491.29 & 9.18 & 9.23\\
\bottomrule
\end{tabular}%

}

% \vspace{0.3em}
% \GCColorbar
% \vspace{0.5em}

\end{table*}


\subsubsection{Diagnostic selection and conditioning variants}

Table~\ref{tab:supplementary-diagnostics_lio} and Table~\ref{tab:supplementary-diagnostics_lpo} report cell-wise LIO and LPO results for three diagnostic variants: learned-only selection with \(\alpha=0\), the prior-heavy configuration \((\gamma,\alpha)=(0.8,0.8)\), and GeoPAS without dimension conditioning $\psi_d(\log(d))$. 
These results complement the main selection-score and ablation analyses. 
The learned-only selector often attains very low medians, but its means and LPO upper tails can become extreme, confirming that instance-conditioned discrimination alone is not mean-safe under heavy-tailed \(\mathrm{relERT}\). 
The prior-heavy setting shows the opposite trade-off: it can reduce the LPO mean below SBS, but does so by moving toward a more conservative, prior-centered selector.
Finally, the no-dimension-conditioning variant preserves typical performance in many cells while producing large mean deteriorations, supporting the interpretation that \(\psi_d(\log d)\) mainly provides global context for far-tail stability rather than ordinary ranking.
% Finally, the no-dimension-conditioning variant preserves typical performance in many cells while producing large mean deteriorations, supporting the interpretation in Section~\ref{subsec:representation-ablation} that \(\psi_d(\log d)\) mainly provides global context for far-tail stability rather than ordinary ranking.

% \begin{figure*}[t]
%     \centering
%     \includegraphics[width=\linewidth]{img/GECCO2026/selection_distribution.pdf}
%     \caption{Selection distributions and pick frequencies (GeoPAS vs.\ VBS) under LIO, Random, and LPO.}
%     \label{fig:selection_details_full}
% \end{figure*}

% \begin{figure*}[t]
%     \centering
%     \includegraphics[width=\linewidth]{img/GECCO2026/survival_curves.pdf}
%     \caption{Survival curves $\mathbb{P}(\mathrm{relERT}>t)$ for GeoPAS and SBS under LIO, Random, and LPO.}
%     \label{fig:survival_curves_full}
% \end{figure*}

% \subsubsection{Failure analysis}\label{app:failure_analysis}
% Figure~\ref{fig:selection_details_full} shows selection distributions and pick frequencies across protocols, and Figure~\ref{fig:survival_curves_full} shows the corresponding survival curves. The broader protocol-wise plots are qualitatively consistent with the main-text analysis: relative to SBS, GeoPAS places more mass in the low-\(\mathrm{relERT}\) region, while the residual failures remain concentrated in a comparatively small subset of selections. The corresponding survival curves show a similar pattern across protocols, with clearer separation through the bulk of the distribution than in the far tail, particularly under LPO. These supplementary plots therefore mainly support the claim that the previously discussed behavior is not specific to a single protocol or visualization.

% \begin{figure*}[t]
%     \centering
%     \includegraphics[width=0.94\linewidth]{img/GECCO2026/performance_heatmap_over_budgets.pdf}
%     \caption{Heatmaps of mean (top), median (middle), and 90th percentile (bottom) $\mathrm{relERT}$ over number of views $k$ and resolution $r$ across protocols.}
%     \label{fig:heatmaps_over_budget_full}
% \end{figure*}

% \subsubsection{Robustness over budget and coarseness}\label{app:robustness_over_budgets}
% Figure~\ref{fig:heatmaps_over_budget_full} shows performance heatmaps over the number of slices $k$ and resolution $r$ (each cell uses $k\cdot r^2$ evaluations). The full protocol-wise plots are consistent with the summary given in the main text. Under LIO and Random, larger budgets tend to improve the median and 90th-percentile statistics, though not in a strictly monotone manner for every configuration. Under LPO, the dependence on budget allocation is less regular: median performance stays within a relatively narrow range across many settings, whereas the mean is more sensitive to particular combinations of the number of views and within-view resolution. This suggests that finer geometric details may not always be beneficial for cross-problem transfer, where the distribution of the probing budget may matter in addition to its total size.
