# Supplementary material for: Geometric Probing for Algorithm Selection in Continuous Black-Box Optimization
Source: arXiv:2604.09095 source file (2026-10-07)
Supplement: Supplementary file 3 [file reframed_table.tex]

\begin{tabular}{cc|cccc|cccc|cccc|cccc|cccc|cccc}
\toprule
\textbf{F. group} & \textbf{D} &
\multicolumn{8}{c|}{\textbf{Mean}} &
\multicolumn{8}{c|}{\textbf{Median}} &
\multicolumn{8}{c}{\textbf{P90}}\\
\cmidrule{3-10}\cmidrule{11-18}\cmidrule{19-26}
& &
\multicolumn{4}{c|}{\textbf{LIO}} &
\multicolumn{4}{c|}{\textbf{LPO}} &
\multicolumn{4}{c|}{\textbf{LIO}} &
\multicolumn{4}{c|}{\textbf{LPO}} &
\multicolumn{4}{c|}{\textbf{LIO}} &
\multicolumn{4}{c}{\textbf{LPO}}\\
\cmidrule{3-6}\cmidrule{7-10}\cmidrule{11-14}\cmidrule{15-18}\cmidrule{19-22}\cmidrule{23-26}
& &
GeoPAS & $\alpha=0$ & $\gamma=.8,\alpha=.8$ & no-$\psi_d$ &
GeoPAS & $\alpha=0$ & $\gamma=.8,\alpha=.8$ & no-$\psi_d$ &
GeoPAS & $\alpha=0$ & $\gamma=.8,\alpha=.8$ & no-$\psi_d$ &
GeoPAS & $\alpha=0$ & $\gamma=.8,\alpha=.8$ & no-$\psi_d$ &
GeoPAS & $\alpha=0$ & $\gamma=.8,\alpha=.8$ & no-$\psi_d$ &
GeoPAS & $\alpha=0$ & $\gamma=.8,\alpha=.8$ & no-$\psi_d$\\
\midrule
\multirow{5}{*}{f1-f5} & 2 & 2.28 & 2.35 & 2.25 & 2.59 & 2.39 & 3.53 & 2.45 & 2.70 & 1.95 & 1.00 & 1.95 & 1.95 & 1.95 & 1.95 & 1.95 & 1.95 & 4.10 & 3.20 & 4.10 & 4.10 & 4.10 & 4.25 & 4.10 & 4.10\\
 & 3 & 14.39 & 54.89 & 60.96 & 142.65 & 343.87 & 4137.15 & 346.21 & 336.73 & 2.64 & 1.13 & 2.64 & 2.64 & 2.64 & 2.64 & 2.64 & 2.64 & 13.68 & 12.26 & 13.68 & 72.09 & 1765.87 & 13407.35 & 1765.87 & 1765.87\\
 & 5 & 11.77 & 20.62 & 11.99 & 12.45 & 19.86 & 1494.66 & 12.09 & 12.34 & 1.64 & 1.06 & 1.64 & 1.64 & 1.82 & 3.22 & 1.82 & 2.00 & 51.82 & 3.79 & 51.82 & 53.15 & 51.82 & 633.14 & 51.82 & 51.82\\
 & 10 & 3.26 & 198.31 & 3.00 & 737.28 & 52.49 & 2596.49 & 3.54 & 492.95 & 2.94 & 1.16 & 2.94 & 2.94 & 2.94 & 4.01 & 2.94 & 2.94 & 6.17 & 7.24 & 5.20 & 7.24 & 7.24 & 1230.70 & 7.24 & 7.24\\
\cmidrule{2-26}
 & all & 7.93 & 69.04 & 19.55 & 223.74 & 104.65 & 2057.95 & 91.07 & 211.18 & 2.03 & 1.05 & 2.39 & 2.23 & 2.64 & 2.74 & 2.64 & 2.62 & 11.55 & 7.14 & 11.76 & 13.68 & 28.96 & 124.72 & 14.31 & 25.76\\
\midrule
\multirow{5}{*}{f6-f9} & 2 & 1.26 & 1.75 & 1.20 & 1.23 & 3.95 & 375.36 & 1.74 & 6.65 & 1.08 & 1.31 & 1.08 & 1.11 & 1.08 & 1.44 & 1.13 & 1.16 & 1.60 & 1.88 & 1.60 & 1.60 & 2.14 & 38.30 & 4.13 & 3.55\\
 & 3 & 1.07 & 3.54 & 1.05 & 1.10 & 674.98 & 1609.17 & 1.57 & 1591.65 & 1.06 & 1.04 & 1.05 & 1.05 & 1.06 & 1.18 & 1.06 & 1.06 & 1.07 & 1.46 & 1.07 & 1.07 & 4.76 & 103.73 & 3.33 & 3.92\\
 & 5 & 1.33 & 1.20 & 1.42 & 1.30 & 2142.51 & 2632.34 & 2.81 & 3792.71 & 1.27 & 1.06 & 1.27 & 1.27 & 1.37 & 1.17 & 1.46 & 1.37 & 1.55 & 1.68 & 2.04 & 1.79 & 12235.31 & 12232.66 & 9.68 & 24460.72\\
 & 10 & 1.36 & 1.30 & 1.58 & 1.30 & 735.43 & 1348.85 & 1.90 & 1713.71 & 1.20 & 1.19 & 1.38 & 1.20 & 1.30 & 1.21 & 1.50 & 1.20 & 1.72 & 1.96 & 2.57 & 1.61 & 3.22 & 1242.55 & 4.07 & 4.35\\
\cmidrule{2-26}
 & all & 1.26 & 1.95 & 1.32 & 1.23 & 889.22 & 1491.43 & 2.01 & 1776.18 & 1.07 & 1.09 & 1.09 & 1.07 & 1.09 & 1.23 & 1.19 & 1.11 & 1.60 & 1.76 & 1.72 & 1.61 & 5.94 & 49.11 & 4.07 & 33.17\\
\midrule
\multirow{5}{*}{f10-f14} & 2 & 1.00 & 1.02 & 1.01 & 1.03 & 1.98 & 54.67 & 2.04 & 2.08 & 1.00 & 1.00 & 1.00 & 1.00 & 1.00 & 1.00 & 1.00 & 1.00 & 1.00 & 1.00 & 1.00 & 1.00 & 3.32 & 2.86 & 4.44 & 4.46\\
 & 3 & 1.03 & 98.85 & 1.05 & 1.12 & 1.69 & 100.01 & 2.69 & 2.14 & 1.00 & 1.00 & 1.00 & 1.00 & 1.00 & 1.00 & 1.78 & 1.01 & 1.01 & 1.01 & 1.01 & 1.01 & 4.84 & 3.07 & 5.82 & 4.84\\
 & 5 & 1.33 & 196.76 & 1.75 & 1.15 & 2.24 & 589.49 & 3.84 & 2.32 & 1.01 & 1.01 & 1.03 & 1.00 & 1.03 & 1.05 & 4.07 & 1.29 & 2.07 & 1.17 & 3.50 & 1.32 & 5.49 & 4.17 & 7.50 & 5.49\\
 & 10 & 1.49 & 196.84 & 1.77 & 1.24 & 51.40 & 3083.57 & 2.75 & 2.10 & 1.09 & 1.01 & 1.10 & 1.00 & 1.50 & 1.24 & 1.79 & 1.13 & 2.80 & 1.36 & 3.83 & 1.50 & 4.97 & 12232.25 & 4.97 & 4.81\\
\cmidrule{2-26}
 & all & 1.21 & 123.37 & 1.40 & 1.14 & 14.33 & 956.94 & 2.83 & 2.16 & 1.00 & 1.00 & 1.00 & 1.00 & 1.01 & 1.01 & 1.37 & 1.03 & 1.37 & 1.27 & 2.69 & 1.13 & 4.88 & 4.01 & 5.49 & 4.85\\
\midrule
\multirow{5}{*}{f15-f19} & 2 & 1.90 & 100.39 & 1.95 & 2.01 & 22.45 & 4283.06 & 21.86 & 112.97 & 1.73 & 1.00 & 1.73 & 1.73 & 2.75 & 4.89 & 2.35 & 2.07 & 3.26 & 1.96 & 3.26 & 3.26 & 86.02 & 24541.29 & 84.64 & 81.45\\
 & 3 & 2.84 & 931.60 & 2.83 & 3.11 & 5.04 & 14778.51 & 3.89 & 101.98 & 2.13 & 1.11 & 2.61 & 2.20 & 3.44 & 12.21 & 3.43 & 2.61 & 3.85 & 3.85 & 3.58 & 5.23 & 11.36 & 36690.30 & 6.35 & 9.38\\
 & 5 & 4.34 & 1029.88 & 4.44 & 3.97 & 103.14 & 8076.31 & 4.91 & 249.44 & 2.23 & 1.05 & 2.23 & 2.23 & 2.33 & 5.20 & 2.23 & 2.28 & 14.86 & 6.74 & 14.86 & 14.86 & 14.86 & 36690.30 & 14.86 & 13.77\\
 & 10 & 2.31 & 637.26 & 2.18 & 246.95 & 148.81 & 7339.63 & 2.16 & 2692.87 & 1.00 & 1.00 & 1.00 & 1.00 & 1.00 & 1.51 & 1.00 & 1.00 & 5.57 & 1.93 & 5.57 & 5.57 & 4.07 & 36690.30 & 5.57 & 18.70\\
\cmidrule{2-26}
 & all & 2.85 & 674.78 & 2.85 & 64.01 & 69.86 & 8619.38 & 8.20 & 789.32 & 1.99 & 1.00 & 2.03 & 1.99 & 2.17 & 3.73 & 2.13 & 2.10 & 5.00 & 3.67 & 5.57 & 5.57 & 13.85 & 36690.30 & 14.79 & 12.83\\
\midrule
\multirow{5}{*}{f20-f24} & 2 & 2.44 & 1.32 & 6.20 & 3.06 & 4.96 & 1568.87 & 12.03 & 23.88 & 1.54 & 1.00 & 1.61 & 1.61 & 1.97 & 2.45 & 7.04 & 5.59 & 3.69 & 1.51 & 12.05 & 7.04 & 12.05 & 9.88 & 12.05 & 126.43\\
 & 3 & 3.14 & 1.38 & 8.11 & 20.83 & 33.95 & 1149.70 & 47.32 & 31.29 & 1.67 & 1.01 & 1.67 & 1.67 & 1.68 & 3.58 & 1.68 & 1.68 & 4.22 & 1.76 & 6.23 & 14.33 & 191.82 & 95.23 & 249.05 & 197.54\\
 & 5 & 1.17 & 1.04 & 1.19 & 1126.46 & 197.05 & 4697.55 & 2.39 & 2888.43 & 1.00 & 1.00 & 1.00 & 1.00 & 1.00 & 1.03 & 1.00 & 1.00 & 1.77 & 1.08 & 1.77 & 1.77 & 3.45 & 24460.96 & 3.45 & 12234.05\\
 & 10 & 1.55 & 50.07 & 1.59 & 197.24 & 4.17 & 7437.03 & 18.49 & 788.21 & 1.00 & 1.00 & 1.00 & 1.00 & 1.00 & 1.00 & 1.48 & 1.16 & 2.19 & 1.32 & 2.19 & 2.19 & 2.94 & 36690.30 & 106.07 & 3.69\\
\cmidrule{2-26}
 & all & 2.07 & 13.45 & 4.27 & 336.90 & 60.03 & 3713.29 & 20.06 & 932.95 & 1.01 & 1.00 & 1.48 & 1.46 & 1.54 & 1.76 & 1.65 & 1.65 & 2.60 & 1.42 & 6.23 & 3.28 & 8.71 & 24462.28 & 77.36 & 73.36\\
\midrule
\multirow{5}{*}{all} & 2 & 1.80 & 22.18 & 2.58 & 2.01 & 7.28 & 1293.84 & 8.29 & 30.62 & 1.46 & 1.00 & 1.52 & 1.46 & 1.64 & 1.74 & 1.80 & 1.82 & 2.92 & 1.95 & 3.26 & 3.26 & 8.79 & 48.83 & 10.43 & 9.82\\
 & 3 & 4.64 & 226.99 & 15.38 & 35.12 & 192.61 & 4469.31 & 83.61 & 363.64 & 1.07 & 1.00 & 1.61 & 1.44 & 1.76 & 2.13 & 1.89 & 1.95 & 5.06 & 2.93 & 5.06 & 5.06 & 11.36 & 25048.82 & 12.20 & 8.24\\
 & 5 & 4.10 & 260.26 & 4.27 & 238.56 & 424.23 & 3534.14 & 5.31 & 1288.89 & 1.09 & 1.01 & 1.23 & 1.05 & 1.32 & 1.64 & 1.68 & 1.60 & 3.88 & 3.10 & 5.12 & 4.45 & 13.13 & 24477.48 & 12.98 & 26.17\\
 & 10 & 2.02 & 225.73 & 2.04 & 246.61 & 176.08 & 4486.63 & 5.93 & 1113.98 & 1.16 & 1.00 & 1.32 & 1.05 & 1.49 & 1.51 & 1.61 & 1.44 & 4.06 & 2.42 & 4.19 & 4.45 & 4.89 & 36690.30 & 5.57 & 5.75\\
\cmidrule{2-26}
 & all & 3.14 & 183.79 & 6.07 & 130.58 & 200.05 & 3445.98 & 25.78 & 699.28 & 1.19 & 1.00 & 1.40 & 1.17 & 1.58 & 1.73 & 1.76 & 1.64 & 3.96 & 2.64 & 4.10 & 4.10 & 7.84 & 24491.29 & 9.18 & 9.23\\
\bottomrule
\end{tabular}%
