# Supplementary material for: Geometric Probing for Algorithm Selection in Continuous Black-Box Optimization
Source: arXiv:2604.09095 source file (2026-10-07)
Supplement: Supplementary file 5 [file results_on_coco_bbob.tex]

\subsection{Dataset and Performance Metric}\label{subsec:dataset}
We evaluate on the COCO/BBOB 2009 single-objective suite~\cite{hansen2009real}, consisting of 24 scalable continuous test functions grouped by properties such as separability, conditioning, and multimodality. 
Each function admits multiple instances via random shifts in decision space and objective space. 
Following the standard AS benchmark protocol of \cite{seiler2025deep}
(building on \cite{kerschke2019automated}), we consider the established
portfolio $\mathcal{A}$ of 12 complementary solvers drawn from COCO
submissions~\cite{hansen2021coco}, covering deterministic baselines
(BSrr~\cite{baudivs2015global}, BSqi~\cite{povsik2015dimension}),
multi-level methods (MLSL, fmincon)~\cite{pal2013comparison},
HMLSL~\cite{pal2013benchmarking}, MCS~\cite{huyer2009benchmarking},
model-based SMAC-BBOB~\cite{hutter2013evaluation},
CMA-ES variants (CMA-CSA~\cite{atamna2015benchmarking}, IPOP400D~\cite{auger2013benchmarking}, HCMA~\cite{loshchilov2013bi}),
and OQNLP~\cite{pal2013comparison}.
Consistent with the same protocol, we use dimensions $d \in \{2,3,5,10\}$ and instances $i \in \{1,2,3,4,5\}$ for each $(f,d)$ pair.

Performance is measured by the \emph{Expected Running Time} (ERT), defined as the expected number of function evaluations required to reach a target value within $\varepsilon=10^{-2}$ of the known optimum:
\begin{equation}
    \mathrm{ERT}(\varepsilon)
    =
    \frac{\sum_{r=1}^{n} \mathrm{FE}_{r}(\varepsilon)}
         {\sum_{r=1}^{n} \mathrm{Succ}_{r}(\varepsilon)},
\end{equation}
where $\mathrm{FE}_{r}(\varepsilon)$ is the evaluation count for run $r$ until the target is reached, $\mathrm{Succ}_{r}(\varepsilon)\in\{0,1\}$ indicates success, and $n$ denotes the number of pooled runs. 
To compare across problems, we use relative ERT
\begin{equation}\label{eq:relert}
\mathrm{relERT}_{f,d,a}
=
\frac{\mathrm{ERT}_{f,d,a}}
     {\min_{a' \in \mathcal{A}} \mathrm{ERT}_{f,d,a'}}.
\end{equation}

Throughout this work, relERT is computed solely from solver ERTs provided by COCO. 
Representation-construction costs are excluded from relERT so that the metric reflects only downstream solver performance under a fixed probing regime; we discuss the practical implications of this additional probing cost in \S\ref{sec:discussion}.

For algorithms whose pooled ERT is undefined because the target is never reached, a PAR10-style penalty is applied by replacing the undefined relERT with ten times the largest finite relERT observed in the benchmark, following \cite{kerschke2019automated}. 
For label construction, we pool the 5 instances of each $(f,d)$ and compute ERT over the resulting runs, yielding 96 labeled $(f,d)$ problems (24 functions $\times$ 4 dimensions), each with one relERT value per algorithm. 
These pooled labels are then paired with instance-level geometric representations constructed from individual problem instances, as described in \S\ref{subsec:geometric-probe}.




\section{Results}
\label{sec:results}


\begin{table*}
\centering
\caption{Results in $\mathrm{relERT}$ across evaluation protocols. GeoPAS cells $(\text{F. group},d)$ are shaded by the fraction of the VBS--SBS gap closed, with closure $\in[0,1]$ mapped to a grayscale in $[0,50\%]$ where darker is better. Non-improving cells are unshaded and denoted $^\dagger$.}
\label{tab:main-results}
% \resizebox{0.95\linewidth}{!}{%
\begin{tabular}{cc|ccc|ccc|ccc}
\toprule
\textbf{F. group} & \textbf{D} & \multicolumn{3}{c}{\textbf{Mean}}&\multicolumn{3}{c}{\textbf{Median}}&  \multicolumn{3}{c}{\textbf{90th percentile relERT}}\\
\cmidrule{3-5}\cmidrule{6-8}\cmidrule{9-11}
 &  &  \textbf{SBS}& LIO& LPO&\textbf{SBS}& LIO& LPO  & \textbf{SBS}& LIO&LPO  \\
\midrule
\multirow{5}{*}{f1-f5} & 2 & 3.71 & \GCCell{26.30}{2.28} & \GCCell{24.25}{2.39} & 2.74 & \GCCell{22.70}{1.95} & \GCCell{22.70}{1.95} & 9.23 & \GCCell{31.15}{4.10} & \GCCell{31.15}{4.10}\\
& 3 & 356.10 & \GCCell{48.10}{14.39} & \GCCell{1.70}{343.87} & 5.06 & \GCCell{29.80}{2.64} & \GCCell{29.80}{2.64} & 1765.87 & \GCCell{49.65}{13.68} & \GCCell{0.00}{1765.87}\\
& 5 & 11.99 & \GCCell{1.00}{11.77} & \GCCell{-35.85}{19.86$^\dagger$} & 1.64 & \GCCell{0.00}{1.64} & \GCCell{-14.20}{1.82$^\dagger$} & 51.82 & \GCCell{0.00}{51.82} & \GCCell{0.00}{51.82}\\
& 10 & 2.74 & \GCCell{-14.95}{3.26$^\dagger$} & \GCCell{-1427.75}{52.48$^\dagger$} & 2.94 & \GCCell{0.00}{2.94} & \GCCell{0.00}{2.94} & 4.01 & \GCCell{-35.70}{6.17$^\dagger$} & \GCCell{-53.55}{7.24$^\dagger$}\\
\cmidrule{2-11}
& all & 93.63 & \GCCell{46.25}{7.92} & \GCCell{-5.95}{104.65$^\dagger$} & 2.84 & \GCCell{22.00}{2.03} & \GCCell{5.50}{2.64} & 13.49 & \GCCell{7.80}{11.55} & \GCCell{-61.90}{28.96$^\dagger$}\\
\midrule
\multirow{5}{*}{f6-f9} & 2 & 5.80 & \GCCell{47.30}{1.26} & \GCCell{19.30}{3.95} & 6.88 & \GCCell{49.30}{1.08} & \GCCell{49.30}{1.08} & 8.29 & \GCCell{45.90}{1.60} & \GCCell{42.20}{2.14}\\
& 3 & 4.46 & \GCCell{48.95}{1.07} & \GCCell{-9695.30}{674.98$^\dagger$} & 4.66 & \GCCell{49.20}{1.06} & \GCCell{49.15}{1.06} & 7.47 & \GCCell{49.45}{1.07} & \GCCell{21.00}{4.76}\\
& 5 & 3.90 & \GCCell{44.25}{1.33} & \GCCell{-100}{2142.51$^\dagger$} & 2.32 & \GCCell{39.65}{1.27} & \GCCell{36.15}{1.37} & 9.68 & \GCCell{46.85}{1.55} & \GCCell{-100}{12235.31$^\dagger$}\\
& 10 & 2.16 & \GCCell{34.55}{1.36} & \GCCell{-100}{735.43$^\dagger$} & 1.78 & \GCCell{37.10}{1.20} & \GCCell{30.60}{1.30} & 4.07 & \GCCell{38.35}{1.72} & \GCCell{13.80}{3.22}\\
\cmidrule{2-11}
& all & 4.08 & \GCCell{45.85}{1.25} & \GCCell{-14376.15}{889.22$^\dagger$} & 3.21 & \GCCell{48.45}{1.07} & \GCCell{47.95}{1.09} & 8.29 & \GCCell{45.90}{1.60} & \GCCell{16.15}{5.94}\\
\midrule
\multirow{5}{*}{f10-f14} & 2 & 6.29 & \GCCell{50.00}{1.00} & \GCCell{40.75}{1.98} & 6.77 & \GCCell{50.00}{1.00} & \GCCell{50.00}{1.00} & 8.20 & \GCCell{50.00}{1.00} & \GCCell{33.90}{3.32}\\
& 3 & 4.98 & \GCCell{49.65}{1.03} & \GCCell{41.35}{1.69} & 4.84 & \GCCell{50.00}{1.00} & \GCCell{50.00}{1.00} & 7.46 & \GCCell{49.90}{1.01} & \GCCell{20.25}{4.84}\\
& 5 & 4.21 & \GCCell{44.90}{1.33} & \GCCell{30.65}{2.24} & 4.07 & \GCCell{49.90}{1.01} & \GCCell{49.55}{1.03} & 7.50 & \GCCell{41.75}{2.07} & \GCCell{15.45}{5.49}\\
& 10 & 2.76 & \GCCell{36.00}{1.49} & \GCCell{-1385.00}{51.40$^\dagger$} & 1.79 & \GCCell{44.10}{1.09} & \GCCell{18.30}{1.50} & 4.97 & \GCCell{27.30}{2.80} & \GCCell{0.00}{4.97}\\
\cmidrule{2-11}
& all & 4.56 & \GCCell{47.05}{1.21} & \GCCell{-137.30}{14.33$^\dagger$} & 4.60 & \GCCell{50.00}{1.00} & \GCCell{49.90}{1.01} & 7.50 & \GCCell{47.15}{1.37} & \GCCell{20.15}{4.88}\\
\midrule
\multirow{5}{*}{f15-f19} & 2 & 25.34 & \GCCell{48.15}{1.90} & \GCCell{5.95}{22.45} & 2.07 & \GCCell{16.15}{1.73} & \GCCell{-31.40}{2.75$^\dagger$} & 118.11 & \GCCell{49.05}{3.26} & \GCCell{13.70}{86.02}\\
& 3 & 2.63 & \GCCell{-6.30}{2.84$^\dagger$} & \GCCell{-73.80}{5.04$^\dagger$} & 2.19 & \GCCell{2.75}{2.13} & \GCCell{-52.15}{3.44$^\dagger$} & 3.45 & \GCCell{-8.30}{3.85$^\dagger$} & \GCCell{-161.65}{11.36$^\dagger$}\\
& 5 & 4.29 & \GCCell{-0.65}{4.34$^\dagger$} & \GCCell{-1500.00}{103.14$^\dagger$} & 2.23 & \GCCell{0.00}{2.23} & \GCCell{-3.95}{2.33$^\dagger$} & 14.86 & \GCCell{0.00}{14.86} & \GCCell{0.00}{14.86}\\
& 10 & 2.02 & \GCCell{-14.45}{2.31$^\dagger$} & \GCCell{-7214.05}{148.81$^\dagger$} & 1.00 & \GCCell{50.00}{1.00} & \GCCell{50.00}{1.00} & 5.57 & \GCCell{0.00}{5.57} & \GCCell{16.45}{4.07}\\
\cmidrule{2-11}
& all & 8.57 & \GCCell{37.80}{2.85} & \GCCell{-404.75}{69.86$^\dagger$} & 2.08 & \GCCell{4.40}{1.99} & \GCCell{-3.95}{2.17$^\dagger$} & 6.50 & \GCCell{13.65}{5.00} & \GCCell{-66.70}{13.85$^\dagger$}\\
\midrule
\multirow{5}{*}{f20-f24} & 2 & 44.95 & \GCCell{48.35}{2.44} & \GCCell{45.50}{4.96} & 10.09 & \GCCell{47.05}{1.53} & \GCCell{44.65}{1.97} & 183.62 & \GCCell{49.30}{3.69} & \GCCell{46.95}{12.05}\\
& 3 & 66.81 & \GCCell{48.40}{3.14} & \GCCell{24.95}{33.95} & 3.05 & \GCCell{33.60}{1.67} & \GCCell{33.40}{1.68} & 249.05 & \GCCell{49.35}{4.21} & \GCCell{11.55}{191.82}\\
& 5 & 7.67 & \GCCell{48.75}{1.17} & \GCCell{-1419.45}{197.05$^\dagger$} & 5.15 & \GCCell{50.00}{1.00} & \GCCell{50.00}{1.00} & 24.40 & \GCCell{48.35}{1.77} & \GCCell{44.75}{3.45}\\
& 10 & 23.64 & \GCCell{48.80}{1.55} & \GCCell{43.00}{4.17} & 4.45 & \GCCell{50.00}{1.00} & \GCCell{50.00}{1.00} & 106.07 & \GCCell{49.45}{2.19} & \GCCell{49.10}{2.94}\\
\cmidrule{2-11}
& all & 35.77 & \GCCell{48.45}{2.07} & \GCCell{-34.90}{60.03$^\dagger$} & 5.68 & \GCCell{49.90}{1.01} & \GCCell{44.25}{1.54} & 113.83 & \GCCell{49.30}{2.60} & \GCCell{46.55}{8.71}\\
\midrule
\multirow{5}{*}{all} & 2 & 17.69 & \GCCell{47.60}{1.80} & \GCCell{31.20}{7.28} & 5.83 & \GCCell{45.25}{1.46} & \GCCell{43.35}{1.64} & 18.33 & \GCCell{44.45}{2.92} & \GCCell{27.50}{8.79}\\
& 3 & 90.43 & \GCCell{47.95}{4.63} & \GCCell{-57.15}{192.61$^\dagger$} & 3.79 & \GCCell{48.80}{1.07} & \GCCell{36.30}{1.76} & 77.36 & \GCCell{47.35}{5.06} & \GCCell{43.20}{11.36}\\
& 5 & 6.52 & \GCCell{21.95}{4.10} & \GCCell{-3785.85}{424.23$^\dagger$} & 2.32 & \GCCell{46.45}{1.09} & \GCCell{37.90}{1.32} & 14.86 & \GCCell{39.60}{3.88} & \GCCell{6.25}{13.13}\\
& 10 & 6.85 & \GCCell{41.30}{2.02} & \GCCell{-1446.20}{176.08$^\dagger$} & 1.80 & \GCCell{40.05}{1.16} & \GCCell{19.80}{1.49} & 5.57 & \GCCell{16.55}{4.06} & \GCCell{7.50}{4.89}\\
\cmidrule{2-11}
& all & 30.37 & \GCCell{46.35}{3.14} & \GCCell{-288.85}{200.05$^\dagger$} & 3.44 & \GCCell{46.10}{1.19} & \GCCell{38.00}{1.58} & 14.86 & \GCCell{39.35}{3.96} & \GCCell{25.35}{7.84}\\
\bottomrule
\end{tabular}%
% }

\vspace{0.3em}
\GCColorbar
\vspace{0.5em}

\end{table*}

\subsection{Main Results Across Evaluation Protocols}
\label{sec:main-results}

Table~\ref{tab:main-results} summarizes GeoPAS under the three evaluation protocols. 
We report mean, median, and 90th-percentile \(\mathrm{relERT}\), since these statistics expose different aspects of a heavy-tailed performance distribution. The mean is the conventional aggregate measure but is sensitive to capped or near-capped failures, the median reflects typical selections, and the 90th percentile measures moderate-tail robustness. 
The SBS statistics are computed on the duplicated held-out evaluation rows by broadcasting that solver’s $\mathrm{relERT}$ to every datapoint. 
Lower values are better, with \(\mathrm{relERT}=1\) corresponding to the VBS by definition.

Under the two within-suite protocols, GeoPAS gives consistent improvements over the SBS across all three statistics. 
Aggregated over all functions and dimensions, the mean decreases from \(30.37\) for SBS to \(3.14\) under LIO and \(3.61\) under Random; the median decreases from \(3.44\) to \(1.19\) and \(1.14\), and the 90th percentile from \(14.86\) to \(3.96\) and \(4.06\), respectively. 
The close agreement between LIO and Random is important: although Random removes the deterministic leave-instance structure, it still yields nearly the same aggregate behavior. 
Thus, within the BBOB suite, the sampled geometric representation provides a stable instance-conditioned signal rather than merely exploiting one particular split construction.

The LPO protocol is qualitatively harder. 
Here the model must transfer to a held-out problem family rather than to another instance of a seen family. 
GeoPAS still improves the median from \(3.44\) to \(1.58\) and the 90th percentile from \(14.86\) to \(7.84\), showing that the representation retains useful ranking information under problem-level transfer. 
However, the mean increases to \(200.05\), far worse than the SBS mean of \(30.37\). 
This separation between improved median/P90 and degraded mean is the central empirical tension of the paper: LPO does not show a broad collapse of ordinary ranking quality, but a failure of mean-safe selection under rare severe tail events. 
We analyze this mechanism explicitly in \S\ref{sec:failure-analysis}.

The cell-wise structure supports the same interpretation. 
For the relatively regular groups \(f6\)--\(f9\) and \(f10\)--\(f14\), GeoPAS obtains medians close to the VBS under all protocols, and LIO/Random also strongly reduce the upper tail. 
For \(f20\)--\(f24\), where the SBS has a large upper-tail loss, GeoPAS reduces the group-level 90th percentile from \(113.83\) to \(2.60\) under LIO, \(2.53\) under Random, and \(8.71\) under LPO. 
These gains indicate that coarse geometric views can be highly informative in multimodal or weakly structured regimes where a single global solver is unsafe.

The remaining failures are not evenly distributed. 
Under LIO and Random, the non-improving cells are limited and show similar structure, mostly affecting means rather than medians. 
Under LPO, mean failures become broader and more severe, including \(f6\)--\(f9\) at \(d=5,10\), \(f10\)--\(f14\) at \(d=10\), \(f15\)--\(f19\) at \(d=5,10\), and \(f20\)--\(f24\) at \(d=5\). 
Yet several of these cells retain near-VBS medians, which again points to extreme solver--problem mismatches rather than uniformly poor selection. 
Overall, Table~\ref{tab:main-results} shows a clear hierarchy of difficulty: LIO and Random characterize strong within-suite behavior, while LPO exposes the tail-risk bottleneck that motivates the subsequent analysis of the selection score and failure distribution.


\begin{table*}[t]
\centering
\caption{Comparison with ELA and Deep-ELA under LIO. Brackets after methods indicate probing budgets. The best $\mathrm{relERT}$ per row is in \textbf{bold}.}
\label{tab:baseline_comparison}
% \resizebox{0.82\linewidth}{!}{%
\begin{tabular}{cc|c|cc|cc|cc|cc|cc|c}
\toprule
\textbf{F. group} & \textbf{D} & \textbf{SBS} &
\multicolumn{2}{c|}{\textbf{ELA (50d)}*} &
\multicolumn{2}{c|}{\textbf{Large (25d)}*} &
\multicolumn{2}{c|}{\textbf{Large (50d)}*} &
\multicolumn{2}{c|}{\textbf{Medium (25d)}*} &
\multicolumn{2}{c|}{\textbf{Medium (50d)}*} &
\textbf{GeoPAS (2048)} \\
 &  &  & RF & MLP & kNN & RF & kNN & RF & kNN & RF & kNN & RF & \\
\midrule

\multirow{5}{*}{f1-f5}
& 2   & 3.71 & 10.41 & 10.59 & 9.24  & 10.30 & 14.26 & 13.87 & 17.57 & 7.57  & 16.38 & 14.77 & \textbf{2.28}\\
& 3   & 356.10 & 1480.68 & 11.87 & 19.94 & 66.76 & 15.29 & 15.54 & \textbf{11.72} & 53.23 & 15.32 & 16.13 & 14.39\\
& 5   & 11.99 & 14.14 & 11.97& 17.70 & 17.31 & 22.88 & 22.81 & 17.50 & 17.85 & 24.18 & 24.01 & \textbf{11.77}\\
& 10  & \textbf{2.74} & 14.64 & 15.27 & 9.54  & 9.53  & 16.45 & 16.28 & - & - & - & - & 3.26\\
\cmidrule{2-14}
& all & 93.63 & 379.97 & 12.43& 14.10 & 25.97 & 17.22 & 17.13 & 15.60 & 26.22 & 18.62 & 18.30 & \textbf{7.93}\\
\midrule

\multirow{5}{*}{f6-f9}
& 2   & 5.80 & 8.51 & 3.72 & 2.65 & 2.87 & 3.49 & 4.25 & 2.69 & 3.37 & 5.70 & 4.08 & \textbf{1.26}\\
& 3   & 4.46 & 8.33 & 3.50 & 2.73 & 3.02 & 3.74 & 3.75 & 2.67 & 2.87 & 3.42 & 3.62 & \textbf{1.07}\\
& 5   & 3.90 & 369.26 & 2.62 & 2.40 & 4.27 & 3.03 & 3.89 & 2.48 & 2.45 & 3.59 & 3.39 & \textbf{1.33}\\
& 10  & 2.16 & 1.62 & 1.76 & 2.40 & 2.43 & 2.64 & 2.71 & - & - & - & - & \textbf{1.36}\\
\cmidrule{2-14}
& all & 4.08 & 96.93 & 2.90 & 2.54 & 3.15 & 3.23 & 3.65 & 2.62 & 2.90 & 4.24 & 3.69 & \textbf{1.26}\\
\midrule

\multirow{5}{*}{f10-f14}
& 2   & 6.29 & 1473.16 & 4.72 & 3.52 & 3.12 & 5.32 & 4.80 & 3.91 & 4.40 & 5.33 & 4.65 & \textbf{1.00}\\
& 3   & 4.98 & 7.07 & 3.82 & 2.69 & 3.48 & 3.72 & 4.81 & 2.59 & 3.53 & 3.85 & 4.02 & \textbf{1.03}\\
& 5   & 4.21 & 150.44 & 3.97 & 3.70 & 4.87 & 4.63 & 6.29 & 3.76 & 3.69 & 4.33 & 4.58 & \textbf{1.33}\\
& 10  & 2.76 & 2.87 & 4.35 & 3.54 & 3.62 & 4.52 & 4.15 & - & - & - & - & \textbf{1.49}\\
\cmidrule{2-14}
& all & 4.56 & 408.38 & 4.21 & 3.36 & 3.77 & 4.55 & 5.01 & 3.42 & 3.88 & 4.50 & 4.42 & \textbf{1.21}\\
\midrule

\multirow{5}{*}{f15-f19}
& 2   & 25.34 & 3.89 & 9.25 & 6.45 & 9.76 & 5.64 & 6.76 & 5.73 & 5.99 & 3.48 & 4.29 & \textbf{1.90}\\
& 3   & 2.63 & 441.96 & 5.06 & 5.15 & 4.63 & 5.20 & 5.00 & 5.36 & 4.83 & 5.12 & 4.20 & \textbf{2.84}\\
& 5   & 4.29 & 1470.28 & 6.81 & \textbf{1.87} & 4.07 & 1.90 & 4.24 & 3.95 & 3.51 & 2.25 & 2.44 & 4.34\\
& 10  & 2.02 & 442.01 & 1.96 & 2.06 & 2.05 & \textbf{1.91}& 2.09 & - & - & - & - & 2.31\\
\cmidrule{2-14}
& all & 8.57 & 589.54 & 5.77 & 3.88 & 5.13 & 3.66 & 4.52 & 5.01 & 4.78 & 3.62 & 3.64 & \textbf{2.85}\\
\midrule

\multirow{5}{*}{f20-f24}
& 2   & 44.95 & 148.39 & 3.32& 3.69 & 5.06 & 3.81 & 7.77 & 3.79 & 8.08 & 3.45 & 14.58 & \textbf{2.44}\\
& 3   & 66.81 & \textbf{1.22} & 2.54 & 30.75 & 12.02 & 4.21 & 25.80 & 2.70 & 4.99 & 7.24 & 6.85 & 3.14\\
& 5   & 7.67 & 1.13 & 1.83 & \textbf{1.08} & 4.73 & 1.15 & 3.71 & 1.72 & 1.43 & 1.57 & 1.96 & 1.17\\
& 10  & 23.64 & 148.01 & 3.25 & 1.73& 11.33 & 1.80 & 12.09 & - & - & - & - & \textbf{1.55}\\
\cmidrule{2-14}
& all & 35.77 & 74.69 & 2.74 & 9.31 & 8.29 & 2.74 & 12.34 & \textbf{2.73} & 4.83 & 4.09 & 7.80 & \textbf{2.07}\\
\midrule

\multirow{5}{*}{all}
& 2   & 17.69 & 342.22 & 6.43 & 5.21 & 6.36 & 6.63 & 7.62 & 6.91 & 5.99 & 6.92 & 8.66 & \textbf{1.80}\\
& 3   & 90.43 & 403.67 & 5.44 & 12.65 & 18.61 & 6.54 & 11.28 & 5.10& 14.35 & 7.14 & 7.10 & \textbf{4.64}\\
& 5   & 6.52 & 402.38 & 5.56 & 5.47 & 7.17 & 6.87 & 8.37 & 6.02 & 5.93 & 7.33 & 7.44 & \textbf{4.10}\\
& 10  & 6.85 & 126.84 & 5.46 & 3.91 & 5.93 & 5.58 & 7.66 & - & - & - & - & \textbf{2.02}\\
\cmidrule{2-14}
& all & 30.37 & 318.78 & 5.72& 6.81 & 9.52 & 6.41 & 8.73 & 6.01 & 8.76 & 7.13 & 7.73 & \textbf{3.14}\\
\bottomrule
\end{tabular}%
% }

\vspace{3pt}
{\footnotesize
Notes: The results for ELA and Deep-ELA (columns marked with *) are from the original publication of Deep-ELA~\cite{seiler2025deep}.}
\end{table*}

\subsection{Comparison with Baselines under LIO}
\label{subsec:deepela}

Table~\ref{tab:baseline_comparison} compares GeoPAS with the published ELA and Deep-ELA results reported in~\cite{seiler2025deep}.
Since these baselines are not rerun in our pipeline and are available only under LIO, and since GeoPAS results are averaged over three independently trained seeds whereas the ELA and Deep-ELA values are reproduced as reported in the original study, the comparison should be read as a community-compatible reference point rather than a fully controlled, cost-normalized study.

Within this setting, GeoPAS gives the strongest aggregate performance among the compared methods. 
On the overall row, its mean \(\mathrm{relERT}\) is \(3.14\), compared with \(30.37\) for SBS and \(5.72\) for the best reported ELA/Deep-ELA baseline. 
GeoPAS is also best on every function-group aggregate row and every dimension-wise aggregate row, indicating that the gain is not driven by a single function class or by the lowest-dimensional cases. 
The particularly low aggregate values on \(f_6\)--\(f_9\) and \(f_{10}\)--\(f_{14}\), \(1.26\) and \(1.21\), respectively, suggest that the geometric slice representation captures solver-relevant structure in regimes where the selected solver can be identified with relatively little ambiguity.

The comparison is not uniformly dominant at the individual-cell level. 
GeoPAS is outperformed in several specific \((f,d)\) regimes, including \(f_1\)--\(f_5\) at \(d=3\), \(f_{15}\)--\(f_{19}\) at \(d=5,10\), and \(f_{20}\)--\(f_{24}\) at \(d=3,5\). 
These exceptions are informative rather than incidental: they indicate that geometric probing is a strong static representation, but not a universal replacement for ELA-style descriptors. 
Overall, the LIO comparison supports the main within-suite claim -- GeoPAS is highly competitive, and often best, under the standard instance-split protocol -- while the remaining cell-wise losses motivate treating geometric and landscape-summary representations as potentially complementary rather than mutually exclusive.


\begin{figure*}[t]
    \centering
    \includegraphics[width=\linewidth]{img/IEEETEC2026_GeoPAS/heatmap_over_log_power_prior_lam_lio_lpo.pdf}
    \caption{Sensitivity heatmaps of GeoPAS to the log-power target-shape parameter \(\gamma\) and prior weight \(\alpha\), under LIO/LPO. The rightmost column in each grid corresponds to the raw-normalized \(\mathrm{relERT}\) being used as the metric. The mean/90th-percentile cells are colored in log-scale for discriminability under multiplicative performance scales.}
    \label{fig:selection-score-log-power}
\end{figure*}

% \begin{figure*}[t]
%     \centering
%     \includegraphics[width=\linewidth]{img/IEEETEC2026_GeoPAS/heatmap_normalized_relERT_over_prior_lam.pdf}
%     \caption{Sensitivity over prior weight \(\alpha\) when the target is raw-scale normalized relERT, \(g_{\mathrm{raw}}(R)=(R-1)/(C-1)\). 
%     Compared with the log-power target, raw normalized relERT emphasizes capped failures but compresses most valid performances, leading to weaker typical-case discrimination and stronger dependence on the empirical prior.}
%     \label{fig:selection-score-norm-relert}
% \end{figure*}

\subsection{Effect of the Selection Score}
\label{sec:selection-score-effect}

We next examine whether the selection score behaves according to its intended decomposition. 
The parameter \(\gamma\) determines how resolution is distributed along the \(\log(\mathrm{relERT})\) scale (Figure~\ref{fig:performance-curves}), while \(\alpha\) controls shrinkage from the learned instance-conditioned estimate toward the algorithm-side empirical prior. 
% Figure~\ref{fig:selection-score-log-power} reports the corresponding sensitivity under LIO and LPO; the Random results are qualitatively similar to LIO and are given in Appendix~\ref{app:random-results}.
Figure~\ref{fig:selection-score-log-power} reports the corresponding sensitivity under LIO and LPO; the Random results are qualitatively similar to LIO and are given in Supplementary Appendix \S{C.1}.

The effect of \(\gamma\) is consistent with the target-geometry interpretation. 
When \(\gamma<1\), the transformed target allocates more resolution to low and moderate \(\mathrm{relERT}\) values, making distinctions among good solvers more visible to the regression head. 
This generally improves median and 90th-percentile performance under LIO, and the same tendency is largely observed under Random. 
However, overly small \(\gamma\) weakens the penalty assigned to high-\(\mathrm{relERT}\) and capped outcomes; the resulting selectors can have excellent typical performance but unstable means. 
Conversely, larger \(\gamma\) shifts sensitivity toward poor outcomes, improving tail aversion in some regions but sacrificing fine-grained discrimination among viable solvers. 
Thus, \(\gamma\) controls a genuine statistical trade-off: it decides whether the model is trained mainly to separate good solvers from each other, or to separate unsafe solvers from the rest.

The effect of \(\alpha\) is orthogonal and equally important. 
For small \(\alpha\), selection is dominated by the learned GeoPAS representation. 
These configurations often achieve very low medians and competitive 90th percentiles, especially under the within-suite protocols, but their means are fragile because a small number of severe mis-selections can dominate the arithmetic average. 
As \(\alpha\) increases, the score shrinks toward the algorithm-side marginal estimate, reducing exposure to globally unsafe algorithms. 
This improves mean robustness in several tail-sensitive regimes, but also moves the selector toward a transformed-metric SBS and therefore reduces instance-specific adaptivity. 
The limiting case \(\alpha=1\) is a prior-only solver ranking under the chosen transformed metric.

This explains why the main configuration \((\gamma,\alpha)=(1,0.5)\) is used as the representative GeoPAS setting. 
It is not selected as the best grid cell. 
Rather, \(\gamma=1\) corresponds to normalized log-\(\mathrm{relERT}\), preserving the natural multiplicative scale of relative optimization performance, and \(\alpha=0.5\) gives a balanced shrinkage score between problem-specific prediction and algorithm-side stability. 
Neighboring configurations show similarly strong within-suite behavior and preserve the LPO median/P90 gains, indicating that the result is not an isolated hyperparameter accident.

The grid also shows that more conservative settings can be mean-safe under LPO. 
For example, prior-heavy configurations such as \((\gamma,\alpha)=(0.8,0.8)\) can reduce the LPO mean below the SBS while keeping the other reported statistics competitive. 
This is important evidence that the GeoPAS scoring family can control extreme tails. 
However, these settings are substantially more prior-centered and less representative of an adaptive geometric selector. 
We therefore report them as sensitivity evidence rather than as the main model.

Finally, the raw-normalized \(\mathrm{relERT}\) alternative, shown as the ``Norm'' column in Figure~\ref{fig:selection-score-log-power}, behaves as expected for a heavily skewed target. 
It emphasizes capped and near-capped values, but compresses most valid solver differences into a narrow numerical range. 
Consequently, it can encode tail exposure but gives a weaker learning signal for ordinary solver ranking. 
This supports using the logarithmic target: the transformation of the performance metric is a decisive part of learning-based AS under heavy-tailed \(\mathrm{relERT}\), consistent with recent concerns about benchmark and metric sensitivity in algorithm selection~\cite{petelin2025pitfalls}.


\begin{table*}[t]
\centering
\caption{Component-wise ablation of feature conditioning and slice-scale sampling. Bold numbers indicate improvements over GeoPAS.}
\label{tab:ablation}
\resizebox{\linewidth}{!}{
\begin{tabular}{l|ccc|ccc|ccc}
\toprule
 \textbf{Model \& ablated items}&\multicolumn{3}{c|}{\textbf{Mean}}&\multicolumn{3}{c}{\textbf{Median}}&\multicolumn{3}{|c}{\textbf{90th percentile}}\\
    \textbf{SBS}& \multicolumn{3}{c|}{30.37} & \multicolumn{3}{c}{3.44}& \multicolumn{3}{|c}{14.86} \\
\cmidrule(lr){2-4}\cmidrule(lr){5-7}\cmidrule(lr){8-10} & LIO& Random&LPO&  LIO&Random& LPO& LIO& Random&LPO\\ 
    \midrule
    \textbf{GeoPAS}& 3.14& 3.61&200.05&  1.19&1.14& 1.58& 3.96& 4.06&7.84\\
    \midrule
    \multicolumn{10}{l}{\textbf{Feature $Z$ components}}\\
    Slice-descriptor $z_i$ removed& 20.81& 18.47& 405.92& 1.36& 1.47& 1.57& 7.26& 7.97&18.33\\
 Slice-conditioning $\psi_{\xi}(\xi_i)$ removed& 26.78& 31.42& 160.65& 1.30& 1.40& 1.71& 4.54& 4.43&9.95\\
    Dimension-conditioning $\psi_d(\log d)$ removed & 130.58& 168.86& 699.28& 1.17& 1.17& 1.64& 4.10& 4.25&9.23\\
    $\psi_{\xi}(\xi_i)$ and $\psi_d(\log d)$ both removed & 101.76& 202.88& 279.94& 1.43& 1.46& 1.71& 4.72& 5.03&9.53\\
    \midrule
    \multicolumn{10}{l}{\textbf{Slice-scale distribution}}\\
 $\log \ell \sim \mathcal{U}(\log \ell_{\min}, \log \ell_{\max}) \rightarrow \ell \sim \mathcal{U}(0.02, 0.7)$ & 8.98& 6.82& 666.35& 1.13& 1.17& 1.61& 4.01& 4.10&10.02\\
 \bottomrule
\end{tabular}
}
\end{table*}

\subsection{Representation Ablations}
\label{subsec:representation-ablation}

Table~\ref{tab:ablation} ablates the representation-side components under the same selection score as Table~\ref{tab:main-results}. 
The tested factors are the visual slice descriptor \(z_i\), learned from the value map and propagated mask; the slice-level conditioning \(\psi_{\xi}(\xi_i)\), which reintroduces scale, range, and IQR information removed by per-slice normalization; the instance-level dimension conditioning \(\psi_d(\log d)\); and the distribution used to sample slice scales.

Removing any representation component generally weakens performance, but the failure patterns differ. 
Removing the visual descriptor \(z_i\) produces the clearest degradation in moderate-tail behavior: the 90th percentile increases from \(3.96/4.06/7.84\) to \(7.26/7.97/18.33\) under LIO/Random/LPO. 
This indicates that the encoded slice geometry carries the main signal for avoiding moderately poor solver choices. 
The LPO median remains almost unchanged, but this should not be read as transfer robustness of the ablated model, since both the LPO mean and P90 deteriorate substantially.
Removing \(\psi_{\xi}(\xi_i)\) strongly worsens the LIO and Random means and moderately degrades the median and 90th percentile. 
Thus, per-slice normalization is useful for making local geometry comparable, but the removed amplitude and scale information remains solver-relevant. 

The strongest asymmetry appears in the dimension-conditioning ablation. 
Removing \(\psi_d(\log d)\) raises the mean from \(3.14/3.61/200.05\) to \(130.58/168.86/699.28\) under LIO/Random/LPO, while the corresponding medians change only from \(1.19/1.14/1.58\) to \(1.17/1.17/1.64\). 
The 90th percentiles also remain comparatively close. 
This indicates that dimension conditioning supplies a low-capacity global context that helps prevent rare high-cost selections.
This is plausible because GeoPAS deliberately represents each problem through two-dimensional normalized restrictions, and similar local slice geometry can occur in different ambient dimensions, while solver behavior may change substantially with \(d\). 
Thus, \(\psi_d(\log d)\) appears to act mainly as a far-tail stabilizer rather than as a median-performance feature.

The scale-sampling ablation gives a smaller but consistent message. 
Replacing log-uniform sampling by uniform sampling over \([0.02,0.7]\) worsens the mean in all protocols and degrades the LPO upper tail, while leaving typical performance comparatively close. 
This supports the use of logarithmic scale sampling, which allocates the probing budget over multiplicative scales rather than over absolute side lengths, as a stabilizing choice.

Overall, the ablations show that GeoPAS is not driven by a single convenience feature. 
The visual descriptor provides the strongest moderate-tail discrimination, slice conditioning supplies broadly useful scale and amplitude context, dimension conditioning mainly reduces exposure to rare severe errors, and log-uniform scale sampling improves robustness by multiplicative scale coverage.

% \begin{figure}[ht]
%     \centering
%     \includegraphics[width=\linewidth]{img/GECCO2026/selection_distribution_lpo.pdf}
%     \caption{Histogram of $\mathrm{relERT}$ distribution of GeoPAS vs.\ SBS under LPO. The $\mathrm{relERT}$ axis is displayed in log-scale.}
%     \label{fig:lpo_relert_dist}
% \end{figure}

\begin{table}[t]
\centering
\caption{Tail quadrant counts under thresholds \(x\in\{q^{\mathrm{SBS}}_{0.9},\mu_{\mathrm{SBS}},1000\}\). 
The thresholds correspond respectively to moderate-tail, mean-relevant, and extreme-tail regimes.}
\label{tab:tail-quadrants}
\resizebox{\linewidth}{!}{
\begin{tabular}{ll|cccc}
 \toprule
 \(x\) & \textbf{Protocol} & \multicolumn{4}{c}{\textbf{\#\(\mathrm{relERT}>x\) (\(\mathrm{Total}=4800\))}} \\
 \cmidrule{3-6}
 & & Neither & SBS only & Both & GeoPAS only \\
 \midrule
 \multirow{3}{*}{\(q^{\mathrm{SBS}}_{0.9}\)}
 & LIO    & 4346& 399& 51& 4\\
 & Random & 4338& 399& 51& 12\\
 & LPO    & 4312& 266& 184& 38\\
 \midrule
 \multirow{3}{*}{\(\mu_{\mathrm{SBS}}\)}
 & LIO    & 4450& 299& 51& 0\\
 & Random & 4450& 299& 51& 0\\
 & LPO    & 4416& 166& 184& 34\\
 \midrule
 \multirow{3}{*}{\(1000\)}
 & LIO    & 4750& 50& 0& 0\\
 & Random & 4750& 49& 1& 0\\
 & LPO    & 4729& 0& 50& 21\\
 \bottomrule
\end{tabular}
}
\end{table}

\begin{figure*}[ht!]
    \centering
    \includegraphics[width=\linewidth]{img/IEEETEC2026_GeoPAS/selection_distribution_with_survival_curves.pdf}
    \caption{Realized \(\mathrm{relERT}\) distributions, overall survival curves, and mean-relevant tail survival curves for GeoPAS and SBS under LIO and LPO. 
    The tail survival curves are restricted to datapoints where GeoPAS exceeds \(\mu_{\mathrm{SBS}}\).}
    \label{fig:selection_dist_with_survival_curves_lio_lpo}
\end{figure*}

\subsection{Failure Analysis}
\label{sec:failure-analysis}

The main unresolved behavior in Table~\ref{tab:main-results} is the separation between LPO median/P90 and LPO mean. 
GeoPAS improves the former but fails sharply in the latter, suggesting that the problem is not ordinary ranking quality, but the severity of a small number of selections. 
We therefore distinguish three tail regimes: the moderate tail at the SBS 90th percentile \(q^{\mathrm{SBS}}_{0.9}\), which is directly related to the reported P90 statistic; the mean-relevant tail at the SBS mean \(\mu_{\mathrm{SBS}}\), which isolates selections large enough to affect the arithmetic mean; and the extreme tail at \(1000\).

Table~\ref{tab:tail-quadrants} first shows that GeoPAS reduces moderate-tail exposure. 
At \(x=q^{\mathrm{SBS}}_{0.9}\), SBS has \(450\) tail cases in each protocol. 
GeoPAS reduces this count to \(55\) under LIO, \(63\) under Random, and \(222\) under LPO. 
Thus, even under problem-level transfer, GeoPAS removes more moderate SBS tail cases than it introduces. 
This explains why the 90th percentile improves under all protocols, including LPO.

The mean-relevant and extreme tails reveal the remaining failure mode. 
At \(x=\mu_{\mathrm{SBS}}\), GeoPAS introduces no new tail cases under LIO or Random, but creates \(34\) GeoPAS-only cases under LPO. 
At \(x=1000\), GeoPAS again introduces no new cases under LIO or Random, whereas LPO contains \(21\) GeoPAS-only extreme events. 
These counts are small relative to the \(4800\) evaluated datapoints, but their magnitudes are large enough to dominate the arithmetic mean, as also visible in Figure~\ref{fig:selection_dist_with_survival_curves_lio_lpo}. 
Therefore, the poor LPO mean is not caused by a broad degradation of GeoPAS selections, but by rare severe errors beyond the range summarized by the median and P90.

The survival curves in Figure~\ref{fig:selection_dist_with_survival_curves_lio_lpo} show the same structure distributionally. 
Over all datapoints, GeoPAS shifts probability mass toward lower \(\mathrm{relERT}\), consistent with its median and moderate-tail gains. 
When restricted to mean-relevant GeoPAS tail selections, however, the LPO curve retains substantial far-tail mass, whereas the LIO tail consists only of cases already tailing under SBS. 
This indicates that the LPO pathology is a tail-severity problem under problem-family shift, not a typical-case failure of the geometric representation. 
% The corresponding Random plots, provided in Appendix~\ref{app:random-results}, follow the LIO pattern and serve as a within-suite sanity check.
The corresponding Random plots, provided in Supplementary Appendix \S{C.1}, follow the LIO pattern and serve as a within-suite sanity check.

\begin{figure}[t]
    \centering
    \includegraphics[width=\linewidth]{img/IEEETEC2026_GeoPAS/selection_frequencies_lio_lpo.pdf}
    \caption{Overall and mean-relevant tail selection frequencies of GeoPAS and VBS under LIO and LPO. 
    Algorithms are ordered by descending VBS selection frequency.}
    \label{fig:selection_frequencies_lio_lpo}
\end{figure}

Finally, Figure~\ref{fig:selection_frequencies_lio_lpo} shows that these failures are solver-specific rather than diffuse. 
GeoPAS selection frequencies are more concentrated than the VBS distribution, and the concentration becomes stronger within the mean-relevant tail. 
Under LPO, the severe cases are associated with a small subset of solver choices, whereas the corresponding VBS selections are more dispersed across the portfolio. 
This is consistent with the shrinkage analysis in \S\ref{sec:selection-score-effect}: stronger representation alone is unlikely to remove all failures if the learned score remains overconfident on algorithms whose risk changes under a held-out problem family.

Overall, the failure mode is precise. 
GeoPAS improves typical and moderate-tail behavior across protocols, including LPO, but it is not yet mean-safe under problem-level transfer. 
Its remaining weakness is rare, solver-specific extreme-tail amplification.

\begin{figure*}[t]
    \centering
    \includegraphics[width=\linewidth]{img/IEEETEC2026_GeoPAS/heatmap_over_budget_0.5_prior_lio_lpo.pdf}
    \caption{Sensitivity to probing budget and slice coarseness under the canonical selection score \((\gamma,\alpha)=(1,0.5)\). 
    Each cell reports \(\mathrm{relERT}\) for \(k\) sampled views at resolution \(r\times r\), corresponding to \(kr^2\) objective evaluations per datapoint.}
    \label{fig:budget-robustness}
\end{figure*}

\subsection{Robustness over Probing Budget and Coarseness}
\label{sec:budget-robustness}

We finally examine how GeoPAS behaves as the probing budget and slice coarseness vary. 
Keeping the selection score fixed at the canonical setting \((\gamma,\alpha)=(1,0.5)\), we vary the number of sampled views \(k\) and the slice resolution \(r\times r\). 
Each datapoint therefore uses up to \(kr^2\) objective evaluations, so the grid separates two aspects of probing: broader coverage through more views, and finer within-slice detail through higher resolution. 
% Figure~\ref{fig:budget-robustness} reports LIO and LPO; the Random results, given in Appendix~\ref{app:random-results}, follow the same qualitative pattern as LIO.
Figure~\ref{fig:budget-robustness} reports LIO and LPO; the Random results, given in Supplementary Appendix \S{C.1}, follow the same qualitative pattern as LIO.

Under LIO, increasing the probing budget improves performance until a clear saturation regime is reached. 
The median approaches \(1.1\), and the 90th percentile falls to around \(4\), once a moderate number of views is available. 
The mean also improves substantially, although less monotonically, reflecting the residual sensitivity of arithmetic averages to rare high-\(\mathrm{relERT}\) selections. 
A notable pattern is that, for comparable evaluation budgets, using more low-resolution views is often preferable to using fewer high-resolution slices. 
This suggests that, in the within-suite setting, broad geometric coverage is more valuable than fine local raster detail: the representation benefits from seeing more regions and orientations of the landscape rather than from over-resolving each individual slice.

The LPO behavior is more constrained. 
Across a wide range of \((k,r)\), the median remains close to \(1.5\)--\(1.7\), and the 90th percentile is usually controlled relative to SBS. 
Thus, the geometric signal is already present at coarse resolutions and does not require very fine slices to support typical problem-family transfer. 
The LPO mean, however, remains highly unstable and shows no reliable monotone improvement with either \(k\) or \(r\). 
This is consistent with \S\ref{sec:failure-analysis}: increasing the amount of probing can improve ordinary ranking, but it does not by itself remove rare severe mis-selections under problem-level shift.

Thus, the main configuration \(k=32,r=8\) should be read as a cost-balanced representative setting: coarse probing already captures useful geometric signal, while the remaining LPO mean failure is primarily a tail-safe selection problem rather than a probe-density problem.

% The main configuration, \(k=32\) and \(r=8\), is therefore a cost-balanced choice rather than the best numerical cell. 
% It uses \(2048\) evaluations per datapoint, gives strong LIO/Random performance, and retains competitive LPO median and 90th-percentile behavior without relying on substantially larger probing budgets. 
% Larger configurations can further improve some within-suite statistics, but the cross-problem mean remains governed by tail safety rather than by probe quantity alone. 
% Additional learned-only sweeps with \(\alpha=0\) show the same point, from the opposite direction, that more probing can yield excellent typical rankings, especially within-suite, but without shrinkage the mean remains fragile. 
% Thus, coarse geometric probing is informative, whereas the remaining robustness bottleneck is calibrated, tail-safe selection rather than simply denser landscape sampling.
